# Supplementary material for: A Unified Framework for Fair Spectral Clustering With Effective Graph Learning
Source: arXiv:2311.13766 source file (2023-11-23)
Supplement: Supplementary file 1 [file appendix0.tex]

We still alternately update the variables corresponding to each subtask to solve \eqref{eq-formulation-3}.  The update of $\mathbf{L}$, $\mathbf{R}$, and $\mathbf{Q}$ is the same as the Algorithm \ref{alg:1}. The main difference is updating $\mathbf{U}$, of which the sub-problem is 
\begin{shrinkfix}
\begin{align}
&\underset{\mathbf{U}}{\min}\;\mu \mathrm{Tr}\left(\mathbf{U}^{\top}\mathbf{L}\mathbf{U}\right) + \gamma \lVert \mathbf{Q} - \mathbf{U}\mathbf{R}\rVert_{\mathrm{F}}^2 \notag\\
    & \mathrm{s.t.}\; \mathbf{U}^{\top}\mathbf{D}\mathbf{U} = \mathbf{I}, \mathbf{F}^{\top}\mathbf{U}= \mathbf{0}. 
    \label{eq-nSC-1}
\end{align}
\end{shrinkfix}
Similarly, we let $\mathbf{U} = \mathbf{Z}\mathbf{Y}$ and rewrite the problem as 
\begin{shrinkfix}
\begin{align}
&
\underset{\mathbf{Y}}{\min}\;\mu\mathrm{Tr}\left(\mathbf{Y}^{\top}\mathbf{Z}^{\top}\mathbf{L}\mathbf{Z}\mathbf{Y}\right) + \gamma \lVert \mathbf{Q} - \mathbf{Z}\mathbf{Y}\mathbf{R}\rVert_{\mathrm{F}}^2\notag\\
&\mathrm{s.t.}\; \mathbf{Y}^{\top}\mathbf{Z}^{\top}\mathbf{D}\mathbf{Z}\mathbf{Y} = \mathbf{I}.
    \label{eq-nSC-2}
\end{align}
\end{shrinkfix}
Since the graph learned by our smoothness model has no isolated nodes due to the $\log$ degree constraint in $Reg(\mathbf{L})$. Therefore, there exists a positive definite matrix $\mathbf{M}$ satisfying $\mathbf{Z}^{\top}\mathbf{D}\mathbf{Z} = \mathbf{M}^2$. We let $\mathbf{Y} = \mathbf{M}^{-1}\widetilde{\mathbf{Y}}$ and have 
\begin{shrinkfix}
\begin{align}
&
\underset{ \widetilde{\mathbf{Y}}^{\top}\widetilde{\mathbf{Y}} = \mathbf{I}}{\min}\;\mu\mathrm{Tr}\left(\widetilde{\mathbf{Y}}^{\top}{\mathbf{M}^{-1}}\mathbf{Z}^{\top}\mathbf{L}\mathbf{Z}\mathbf{M}^{-1}\widetilde{\mathbf{Y}}\right) \notag\\
&\;\;\;\;\;\;\;\;\;\;\;+ \gamma \lVert \mathbf{Q} - \mathbf{Z}\mathbf{M}^{-1}\widetilde{\mathbf{Y}}\mathbf{R}\rVert_{\mathrm{F}}^2 \notag\\
\Rightarrow & 
\underset{ \widetilde{\mathbf{Y}}^{\top}\widetilde{\mathbf{Y}} = \mathbf{I}}{\min}\;\mu\mathrm{Tr}\left(\widetilde{\mathbf{Y}}^{\top}{\mathbf{M}^{-1}}\mathbf{Z}^{\top}\mathbf{L}\mathbf{Z}\mathbf{M}^{-1}\widetilde{\mathbf{Y}}\right) \notag\\
&\;\;\;\;\;\;\;\;\;\;\;- 2\gamma \mathrm{Tr}(\mathbf{R}\mathbf{Q}^{\top}\mathbf{Z}\mathbf{M}^{-1}\widetilde{\mathbf{Y}}).
    \label{eq-nSC-3}
\end{align}
\end{shrinkfix}
Let $\widetilde{\phi}(\mathbf{Y})$ be the objective function of \eqref{eq-nSC-3}, which  is differential, and $ 
\nabla_{\widetilde{\mathbf{Y}}}\,\widetilde{\phi}(\widetilde{\mathbf{Y}}) = 2\mu \mathbf{M}^{-1}\mathbf{Z}^{\top}\mathbf{L}\mathbf{Z}\mathbf{M}^{-1}\mathbf{Y}  - 2\gamma \mathbf{M}^{-1}\mathbf{Z}^{\top}\mathbf{Q}\mathbf{R}^{\top}$. Thus, the problem can be solved via the algorithm in \cite{wen2013feasible}.

\begin{comment}
\end{comment}
