# Supplementary material for: A Unified Framework for Fair Spectral Clustering With Effective Graph Learning
Source: arXiv:2311.13766 source file (2023-11-23)
Supplement: Supplementary file 2 [file appendix1.tex]

First, we provide the following lemma.
\begin{lemma}
    The regularizer $Reg_w(\mathbf{w})$ is $4\beta-$strongly convex.
    \label{lemma-regularizer}
\end{lemma}
\begin{proof}
For any $\mathbf{w}\geq 0$, we can calculate the Hessian matrix of $Reg_w(\mathbf{w})$ as $\nabla_{\mathbf{w}\mathbf{w}}Reg_w(\mathbf{w}) = 4\beta \mathbf{I} + \alpha \mathbf{S}^{\top}\mathrm{diag}\left((\mathbf{S}\mathbf{w})^{.(-2)}\right)\mathbf{S}$. We can check that $\nabla_{\mathbf{w}\mathbf{w}}Reg_w(\mathbf{w}) \succ 4\beta \mathbf{I}$. Hence, $Reg_w(\mathbf{w})$ is $4\beta-$strongly convex.
\label{proof-lemma-regularizer}
\end{proof}
Then, according to the definition of $\widehat{\mathbf{L}}$,  we have
\begin{shrinkfix}
\begin{align}
    &\frac{1}{N}\mathrm{Tr}(\mathbf{X}^{\top}\widehat{\mathbf{L}}\mathbf{X}) + Reg(\widehat{\mathbf{L}}) + \mu \mathrm{Tr}(\widehat{\mathbf{U}}^{\top}\widehat{\mathbf{L}}\widehat{\mathbf{U}}) \notag\\ 
    \leq &\frac{1}{N}\mathrm{Tr}(\mathbf{X}^{\top}{\mathbf{L}}^*\mathbf{X}) + Reg({\mathbf{L}}^*) + \mu \mathrm{Tr}(\widehat{\mathbf{U}}^{\top}{\mathbf{L}}^*\widehat{\mathbf{U}})\notag\\
    \Rightarrow& Reg(\widehat{\mathbf{L}}) - Reg({\mathbf{L}}^*) \leq \mathrm{Tr}\left( ({\mathbf{L}}^* -\widehat{\mathbf{L}} ) \left(\frac{1}{N}{\mathbf{X}\mathbf{X}^{\top}} +\mu \widehat{\mathbf{U}}\widehat{\mathbf{U}}^{\top}\right)\right)\notag \\
    \Rightarrow & Reg(\widehat{\mathbf{L}}) - Reg({\mathbf{L}}^*) \leq \left\lVert  \widehat{\mathbf{L}} - {\mathbf{L}}^*\right\rVert_{\mathrm{F}} \left\lVert\frac{1}{N}{\mathbf{X}\mathbf{X}^{\top}}  +\mu \widehat{\mathbf{U}}\widehat{\mathbf{U}}^{\top} \right\rVert_{\mathrm{F}}
    \label{eq-theory-1}
    \end{align}
\end{shrinkfix}
We focus on $Reg$ and have
\begin{shrinkfix}
\begin{align}
 &Reg(\widehat{\mathbf{L}}) - Reg({\mathbf{L}}^*) \notag\\
 =& Reg_w(\widehat{\mathbf{w}}) - Reg_w({\mathbf{w}}^*) \notag\\
\geq& \left\langle \nabla_{\mathbf{w}} Reg_w({\mathbf{w}}^*),  \widehat{\mathbf{w}} - {\mathbf{w}}^*  \right\rangle+ 2\beta \left\lVert \widehat{\mathbf{w}}- {\mathbf{w}}^* \right\rVert_2^2\notag\\
    \geq &  -\left \lVert \nabla_{\mathbf{w}} Reg_w({\mathbf{w}}^*) \right\rVert_2 \left\lVert  \widehat{\mathbf{w}} - {\mathbf{w}}^*\right\rVert_2 + 2\beta \left\lVert\widehat{\mathbf{w}} - {\mathbf{w}}^* \right\rVert_2^2 \notag\\
    \geq&  -C_R \left\lVert  \widehat{\mathbf{w}} - {\mathbf{w}}^*\right\rVert_{2} + 2\beta \left\lVert  \widehat{\mathbf{w}} - {\mathbf{w}}^*\right\rVert_{2}^2,
    \label{eq-theory-2}
    \end{align}
\end{shrinkfix}
where $\widehat{\mathbf{w}}$ and ${\mathbf{w}}^*$ are the upper triangle variables of $\widehat{\mathbf{L}}$ and ${\mathbf{L}}^*$, respectively. The first inequality holds due to Lemma \ref{lemma-regularizer}. The second inequality holds due to triangle inequality. The last inequality holds due to Assumption \ref{assump-r}. Besides, we have 
\begin{shrinkfix}
\begin{align}
\lVert \widehat{\mathbf{L}} - {\mathbf{L}}^*\rVert_{\mathrm{F}} 
 = &\lVert( \widehat{\mathbf{D}} - {\mathbf{D}}^*) - ( \widehat{\mathbf{W}} - {\mathbf{W}}^*)\rVert_{\mathrm{F}} \notag\\
\leq &\lVert \widehat{\mathbf{D}} - {\mathbf{D}}^*\rVert_{\mathrm{F}} + \lVert \widehat{\mathbf{W}} - {\mathbf{W}}^*\rVert_{\mathrm{F}}\notag\\
 =& \lVert \mathbf{S}\widehat{\mathbf{w}} - \mathbf{S}{\mathbf{w}}^*\rVert_{\mathrm{2}} + \sqrt{2}\lVert \widehat{\mathbf{w}} - {\mathbf{w}}^*\rVert_{\mathrm{2}}\notag\\
 \leq & \lVert \mathbf{S}\rVert_{\mathrm{2}} \lVert \widehat{\mathbf{w}} -{\mathbf{w}}^*\rVert_{\mathrm{2}} + \sqrt{2}\lVert \widehat{\mathbf{w}} - {\mathbf{w}}^*\rVert_{\mathrm{2}}\notag\\
 \leq & \left(\sqrt{2(D-1)} + \sqrt{2}\right) \lVert \widehat{\mathbf{w}} - {\mathbf{w}}^*\rVert_{\mathrm{2}}\notag \\
 :=& C_D \lVert \widehat{\mathbf{w}} - {\mathbf{w}}^*\rVert_{\mathrm{2}},
    \label{eq-theory-2-1}
    \end{align}
\end{shrinkfix}
where the last inequality holds due to the spectral norm of $\mathbf{S}$ is $\sqrt{2(D-1)}$. Bringing  \eqref{eq-theory-2-1} and \eqref{eq-theory-2} back to \eqref{eq-theory-1}, we have 
\begin{shrinkfix}
\begin{align}
& 2\beta \left\lVert  \widehat{\mathbf{w}} - {\mathbf{w}}^*\right\rVert_{2}^2 -C_R \left\lVert  \widehat{\mathbf{w}} - {\mathbf{w}}^*\right\rVert_{2}\notag\\
\leq &C_D \lVert \widehat{\mathbf{w}} - {\mathbf{w}}^*\rVert_{\mathrm{2}}\left\lVert\frac{1}{N}\mathbf{X}\mathbf{X}^{\top} +\mu \widehat{\mathbf{U}}\widehat{\mathbf{U}}^{\top} \right\rVert_{\mathrm{F}}\notag\\ 
=& C_D \lVert \widehat{\mathbf{w}} - {\mathbf{w}}^*\rVert_{\mathrm{2}}\notag\\ &\sqrt{\frac{1}{N^2}\mathrm{Tr}\left(\mathbf{X}\mathbf{X}^{\top}\mathbf{X}\mathbf{X}^{\top} \right) + \frac{2\mu}{N}\mathrm{Tr}\left(\mathbf{X}\mathbf{X}^{\top} \widehat{\mathbf{U}}\widehat{\mathbf{U}}^{\top}\right)  + \mu^2\mathrm{Tr}\left(\widehat{\mathbf{U}}\widehat{\mathbf{U}}^{\top}\widehat{\mathbf{U}}\widehat{\mathbf{U}}^{\top}\right)} \notag\\
= &C_D \lVert \widehat{\mathbf{w}} - {\mathbf{w}}^*\rVert_{\mathrm{2}}  \sqrt{C_X+ \frac{2\mu}{N}\mathrm{Tr}\left(\mathbf{X}\mathbf{X}^{\top} \widehat{\mathbf{U}}\widehat{\mathbf{U}}^{\top}\right)  + \mu^2K}\notag\\
=& C_D \lVert \widehat{\mathbf{w}} - {\mathbf{w}}^*\rVert_{\mathrm{2}}  \sqrt{C_X+ \frac{2\mu}{N}\mathrm{Tr}\left(\widehat{\mathbf{Y}}^{\top} \left(\mathbf{Z}^{\top}{\mathbf{X}}{\mathbf{X}}^{\top}{\mathbf{Z}}\right) \widehat{\mathbf{Y}}\right)  + \mu^2K}
    \label{eq-theory-3}
    \end{align}
\end{shrinkfix}
where the second equality holds since $\widehat{\mathbf{U}}^{\top}\widehat{\mathbf{U}} = \mathbf{I}$.
Based on \eqref{eq-theory-3}, we have 
\begin{shrinkfix}
\begin{align}
&\lVert \widehat{\mathbf{L}} - {\mathbf{L}}^*\rVert_{\mathrm{F}} \leq C_D  \left\lVert  \widehat{\mathbf{w}} - {\mathbf{w}}^*\right\rVert_{2} \notag\\
\leq &\frac{C_RC_D}{2\beta} + \frac{C_D^2}{2\beta} \sqrt{C_X+ \frac{2\mu}{N}\mathrm{Tr}\left(\widehat{\mathbf{Y}}^{\top} \left(\mathbf{Z}^{\top}{\mathbf{X}}{\mathbf{X}}^{\top}{\mathbf{Z}}\right) \widehat{\mathbf{Y}}\right)  + K\mu^2},
    \label{eq-theory-4}
    \end{align}
\end{shrinkfix}

Finally, we complete the proof.

% Therefore, the upper error bound is determined by $\mathrm{Tr}\left(\mathbf{X}\mathbf{X}^{\top} \widehat{\mathbf{U}}\widehat{\mathbf{U}}^{\top}\right)$. Furthermore, due to the constraints of $\widehat{\mathbf{U}}$, i.e., $\widehat{\mathbf{U}}^{\top}\widehat{\mathbf{U}} =\mathbf{I}, \mathbf{F}\widehat{\mathbf{U}} = \mathbf{0}$, we define $\widehat{\mathbf{U}} = \mathbf{Z}\widehat{\mathbf{Y}}$. It is not difficult to have that 
% \begin{shrinkfix}
% \begin{align}
% &\mathrm{Tr}\left(\mathbf{X}\mathbf{X}^{\top} \widehat{\mathbf{U}}\widehat{\mathbf{U}}^{\top}\right) = \left \lVert \mathbf{X}^{\top} \widehat{\mathbf{U}}\right \rVert_{\mathrm{F}}^2 =  \left \lVert \mathbf{X}^{\top} \mathbf{Z} \widehat{\mathbf{Y}}\right \rVert_{\mathrm{F}}^2 \notag\\
% &= \mathrm{Tr} \left(\widehat{\mathbf{Y}}^{\top} \left(\mathbf{Z}^{\top}\widehat{\mathbf{X}}\widehat{\mathbf{X}}^{\top}{\mathbf{Z}}\right) \widehat{\mathbf{Y}} \right), \; \mathrm{s.t.}\, \widehat{\mathbf{Y}}^{\top} \widehat{\mathbf{Y}} = \mathbf{I}
%     \label{eq-theory-5}
%     \end{align}
% \end{shrinkfix}
% Next, we will explore the condition of  $\mathrm{Tr}\left(\mathbf{X}\mathbf{X}^{\top} \widehat{\mathbf{U}}\widehat{\mathbf{U}}^{\top}\right)$ reaching its minimum.
